# Supplementary material for: Dynamics of a Persistent Insulator-to-Metal Transition in Strained Manganite Films
Source: arXiv:1906.10334 source file (2019-07-03)
Supplement: Supplementary file 1 [file Supplement_Extras.tex]

For static reflectivity measurements, the sample was illuminated with a broadband white light source focused to a $\sim$100 $\mu$m spot and the reflected light was directed into a spectrometer (ocean optics USB4000). The sample was excited with single laser pulses from an amplified Ti:Sapphire laser isolated with a Pockels cell and a shutter. Single-shot measurements were carried out using a dual-echelon single-shot setup\cite{Shin2014}. A non-collinear OPA generated probe wavelengths between 750 and 540 nm, while the fundamental of the laser was used as a probe at 800 nm. The excitation was the fundamental out of the laser, with a pulse duration of approximately 70 fs. The probe pulse duration is approximately 35 fs, and the overall time resolution of the instrument is less than 100 fs. For experiments with the fundamental, the excitation was cross-polarized relative to the probe to avoid scattered light. The angle of incidence of the pump on the sample was approximately 30 degrees, and the probe as at 45 degrees at the center of the echelons. Conventional pump-probe measurements were carried out using the same 1 kHz amplified system, broadened using a gas tube filled with 250 kPa of argon, and recompressed to a 35 fs pulse, yielding an overall experimental time resolution of 50 fs.

\subsection{Ginzberg-Landau Free Energy Model}

Ginzberg-Landau Model

In the Ginzburg-Landau model of phase transitions, a material with two competing order parameters with biquadratic coupling can be described by a parameterized free energy surface, as described in \color{red}{[}citation{]}\color{black}. We can introduce a coupling of the lattice order parameter to the epitaxial strain. This coupling is linear, as the energy of the charge-ordered state is directly proportional to the strain.

\begin{equation}
G=a\left(\frac{T-T_{co}}{T_{co}}\right)L^{2}+bL^{4}+c\left(\frac{T-T_{C}}{T_{C}}\right)M^{2}+dM^{4}+eM^{2}L^{2}
\end{equation}

In this free energy, surface, in the absence of epitaxial strain,
the global minimum of $G$ is at$L=0$, in the ferromagnetic phase.
In the prescience of a sufficiently large amount of strain, the global
minimum of G is shifted to $M=0$, and L is nonzero. This occurs in
LCMO/NGO films thinner than \textasciitilde{}45 nm. A metastable ferromagnetic
phase may occur when there is an activation barrier between the charge-ordered
and ferromagnetic phases. This requires the magnetoelastic coupling,
$e$, to be sufficiently strong. In this case, there is a metastable
magnetic phase where$L=0$, and a stable charge-ordered phase where
M =0. Excited State Strictly, coherent motion in the excited state
cannot be accommodated by a mean-field thermodynamic potential. However,
because the charge-transfer excitations in manganites are long-lived,
the stability of the photoswitching process may be approximated by
a thermodynamic model. The system has enough time to sample the configuration
space in the ns-s time it takes for the charge-transfer excitations
to relax. Charage transfer excitations will affect . This excitation
process is often referred to as \textquotedblleft charge-order melting\textquotedblright{}
even if thermal heating is not the mechanism for the partial loss
of charge order. Using the effective medium model presented above,
we can model the excited state by modifying the effective charge ordering
temperature, Tco. The charge-ordering order parameter, L, is proportional
to the number of unexcited charge-transfer excitations in the material.
Therefore, $L(X_{e})=L(X_{e}=0)(1-X_{e})$ Solving for the effective
lattice parameter, we obtain for the CO ground state $L^{2}=A(T-T_{c}o)/2B$
and therefore for the excited state, and for the CO excited state,

\begin{equation}
L^{2}(X_{e})=(1-X_{e})^{2}A(T-T_{co})/2
\end{equation}

B since A, B, and T are unchanged, and only TCO changes, 

\begin{equation}
\frac{A(T-T_{co}(X_{e}))}{2B}=\frac{(1-X_{e})^{2}A(T-T_{co})}{2B}
\end{equation}

 solving for 
 
\begin{equation}
T_{co}(X_{e})T_{co}(X_{e})=\left[T-(1-X_{e})\right]{}^{2}(T-T_{co})
\end{equation}

In the absence of strong electron-phonon coupling, the lattice temperature T does not change much, so the temperature of the free energy surface remains mostly unchanged. At some excitation level Xe, the barrier between the magnetic and charge-ordered phases disappears in the excited state. At a lower excitation threshold, the initial energy deposited into the system is higher than the barrier required to cross into the magnetic phase. This excitation level is plotted . Note that the result, Xe = 0.24, agrees well with experimental results of the switching threshold, which place Xe = 0.25 as the critical excited charge-transfer excitation density. The free energy surface is symmetric about M = 0 (and in the absence of strain, is symmetric about L) so we will concern ourselves only with the saddle point in the first quadrant, where M and L are positive, and the charge-ordered phase is enhanced in the presence of strain. The temperature at which switching reverses is when the free energy surface has no activation barrier between the ferromagnetic and charge ordered phases (that is, the curvature of the free energy surface at the saddle point is zero). As a function
of the parameters of the free energy surface, this occurs when
\begin{equation}
\nabla^{2}G=0
\end{equation}
at the saddle point. In this picture, the switching threshold is also
strain-dependent. It is important to note that the free energy surface
that the excited state sees is different than the free energy surface
of the ground state. The CO phase is not accessible by thermal heating, so raising the temperature will never shift the global minimum to the FM phase. In order to switch into the FM phase, the free energy surface must be modified so that the material has enough energy to cross the barrier between the FM and CO phase, and the FM phase must be a global minimum. This corresponds to a specific density of charge-transfer excitations such that the CO lattice parameter, L is weakened. In our model of charge-transfer excitations self-stabilizing by coupling to nearby charge-transfer excitations, this is a mean-field treatment of the charge-transfer interaction. Note that because this is a mean-field model, it is unable to model the effects of domain formation or local correlations. It implicitly assumes that every charge-transfer excitation
is self-stabilized by the average number of charge-transfer excitations in the system.

% \begin{figure}
% \caption{Ginzburg-Landau free energy surface with biquadtracic coupling. Clockwise
% from top left. Free energy surface of the ground state, along with
% the minimum energy path (collective reaction coordinate) to the magnetic
% state. Selected excitation levels, the ground state (blue) the lowest
% level where the excited state energy at L0 is equal to the barrier
% height, and a higher-lying state where the initial energy is greater
% than the barrier height. The barrier height and initial potential
% energy (relative to the equilibrium CO energy in the excited state)
% as a function of the excitaiton density Xe. The switching threshold
% is when KE = V, at Xe = 0.25. Thermal Heating In addition to the dynamics
% of the electronic phase transition, the excitation pulse deposits
% a significant amount of energy into the LCMO film as heat, which must
% be dissipated. The final temperature T2 at a sample depth z below
% the switching threshold can be given by }
% \end{figure}

\begin{equation}
(1-R)Fe^{-z/\delta}=\intop_{T_{1}}^{T_{2}}dT^{'}C_{b}(T^{'})
\end{equation}

With an initial temperature $T_{1}$. Above the switching threshold, the first-order phase transition takes a finite amount of free energy, so additional fluence past the switching threshold. does not increase the temperature as much. According to this model, a fluence of 2 mJ/cm2 (just below the switching threshold for the 36 nm film) produces a final temperature of 170 K. This is above the 130 K threshold for reversal of the ferromagnetic phase. This implies heat transport through the substrate away from the LCMO film is crucial to stabilizing the ferromagnetic phase, and/or the charge-transfer excitations never fully thermalize, even over the nanosecond timescales required to form a phase-separated metallic phase. Both are hypotheses consistent with the literature. Ultrafast electron diffraction measurements with an initial excitation fluence of 4 mJ/cm2 measured a lattice temperature jump of less than 10 K, indicating the excited state is highly nonthermal, and most of the 1.5 eV photon energy is not converted to thermal motion. Pump-probe results on the change in reflectivity in this systems and elsewhere are not consistent with the reflectivity change associated with a temperature jump of this mangnitude.
